# Supplementary material for: User Decision Guidance with Selective Explanation Presentation from Explainable-AI
Source: arXiv:2402.18016 source file (2024-05-27)
Supplement: Supplementary file 1 [file 99_appendix.tex]

\if0
\appendix
\section{Research Methods}
appendix
\fi
